# Supplementary material for: Learning to Walk Autonomously via Reset-Free Quality-Diversity
Source: arXiv:2204.03655 source file (2022-04-07)
Supplement: Supplementary file 1 [file appendix.tex]

% \section{Research Methods}

% \subsection{Part One}

% fff

% \subsection{Part Two}

% \section{Online Resources}

% Nam id fermentum dui. Suspendisse sagittis tortor a nulla mollis, in
% pulvinar ex pretium. Sed interdum orci quis metus euismod, et sagittis
% enim maximus. Vestibulum gravida massa ut felis suscipit
% congue. Quisque mattis elit a risus ultrices commodo venenatis eget
% dui. Etiam sagittis eleifend elementum.
